# Supplementary material for: Asymmetric Image Retrieval with Cross Model Compatible Ensembles
Source: arXiv:2303.17531 source file (2023-10-29)
Supplement: Supplementary file 1 [file implementation_details.tex]

\section{Experiment details}
\label{sec:implementation_details}
In this section we provide additional details on the experiments described in Section 4 of the main paper.

\subsection{Implementation details}
To train the embedding models (either for gallery or query usage), we used three well-known architectures: ResNet18, ResNet100~\cite{he2016deep} and MobileFaceNet~\cite{schroff2015facenet}.
The networks were trained with a \emph{CosFace}~\cite{wang2018cosface} loss function and 512-dimensional embedding space. 

To train the transformation models either for the model2model approach or the unified-space approach, we follow Wang~\etal~\cite{wang2020unified} and implemented the transformation models as RBT modules (more information in~\cite{wang2020unified}).
For both approaches, we used the loss function described in Section 3 of Wang~\etal~\cite{wang2020unified}.

All embedding models and transformation models were trained using the VGG-FACE2 dataset~\cite{Cao2018VGGFace2AD}.
Note that similar to previous work, the training dataset images are available for training as opposed to data used for querying and indexing, which adheres to data retention policies.
In a practical use case, involving production and training infrastructure, the training data may be obtained through data collection while the data used for querying and indexing is the actual data adhering to the retention policies. 

% Following previous works, the training dataset images are available for training as opposed to data used for querying and indexing, which adheres to data retention policies.

\subsection{IJB-C Evaluation protocols}
As described in the main text, we evaluate the visual search methods described in the paper, and in other baselines using the IJB-C benchmark, which contains ~130k images from 3,531 identities.
We used the common testing protocols for face recognition, 1:1 verification and 1:N open-set search, test 1 and test 4 IJB-C protocols respectively.
% The 1:N protocol includes two different gallery sets, and a single query set.
Since the 1:N protocol (test 4) includes two gallery sets, we evaluated the FRR@FAR=1\% results for each gallery individually, and reported the average of these results.
%In the uncertainty section (Section 4.5 in the main paper) we used only a single gallery (gallery 1) of the IJB-C 1:N protocol.
In the uncertainty experiments (Section 4.5 in the main paper) only a single gallery set (gallery 1) was used.
%In the uncertainty section (Section 4.5 in the main paper) we used only a single gallery (gallery 1) of the IJB-C 1:N protocol.

% \subsection{Risk coverage curve}
% In Section 4.5 we propose to use the ensemble of gallery models as a tool for measuring the uncertainty of a gallery embedding.
% To evaluate the uncertainty, we measure the variance between the predictions of the different models in the ensemble. 
% In Fig. 8, we show the error decrease gained by filtering out gallery embeddings with high uncertainty.
% The curve is evaluated by iterating over the gallery 1 images from the IJB-C 1:N protocol, and in each iteration, omitting the gallery image that induces the highest uncertainty.
